# Supplementary material for: Quantum sensing in the fractional Fourier domain
Source: arXiv:2405.03896 source file (2024-05-06)
Supplement: Supplementary file 1 [file Supplemental_Material.pdf]

# Supplemental Material

## CONTENTS


I. Materials and Methods 2
A. Experiment 2
B. Data Analysis 3

II. Rationalization of sufficient conditions for which $\left|\Phi_j^{(\alpha)}\right|^2 \approx (4/\pi)^2 |\sin\alpha| \, |\mathcal{F}_\alpha[g](f_j \sin\alpha)|$ 4

III. Derivation of the second moment of $\Phi$ in relation to $W_g$ for stochastic $g$ 13

IV. Time-frequency illustration of the experimental measurement 14

References 15

# I. MATERIALS AND METHODS

## A. Experiment

An electronic-grade diamond substrate with a 1-micron 12C-enriched (99.99%) overgrown layer (QuantumDiamonds Gmbh) was implanted (Innovion) with 15N ions at 5 keV, 7° tilt, and high fluence $3 \times 10^{13}$ cm$^{-2}$ to create a dense, shallow ensemble of substitutional nitrogen atoms. To prepare the NVs, the diamond was subsequently vacuum annealed at 800° C, washed in piranha solution, oxygen annealed, then washed again in piranha. Just before mounting the diamond was cleaned in an equal-parts mixture of nitric, perchloric, and sulfuric acid.

Experiments were conducted on a custom-built confocal microscope based on a PInano Stage Platform System (Physik Instrumente). A 532-nm laser of intensity $\sim$ 2.5 W/cm$^2$ (Lighthouse Photonics, Sprout G) was used to polarize and read out an NV ensemble located within an approximately diffraction-limited spot. An acousto-optic modulator (G&H AOM, model 3250-220) was used to gate the laser. The laser was focused onto the diamond using a 100x/NA 0.85 air objective lens (Nikon CFI Plan LWD IMSI 100X). Fluorescence from the NVs was collected back through the objective and filtered through a dichroic mirror (Semrock, Di03-R532-t1-25x36), long-pass filter (Semrock, BLP01-635R-25), and 532-notch filter (Semrock, NF01-532U-25) before detection using a single-photon-counting module (Excelitas, SPCM-AQRH-14-ND). Data was acquired using a DAQ unit (NI PCIe-6351). NVs were coherently driven at Rabi frequencies in the range of 10-25 MHz by microwaves generated by an SRS SG384 unit with built-in IQ modulation. Microwaves were gated with a high-speed switch (Mini-Circuits ZASWA2-50DR-FA), amplified (Mini-Circuits ZHL-16W-43-S+), then delivered to the NVs via a small ($\sim$mm) loop. A neodymium magnet (K&J Magnetics) mounted near the diamond was used to set the bias field. An arbitrary waveform generator (RIGOL, DG1022Z) was used to synthesize chirped RF signals of the form:

$$g(t) = A \cos\left[2\pi t \left(\frac{-q_1}{2} t + f_1\right)\right] \text{rect}\left(\frac{t - T/2}{T}\right), \tag{S1}$$

with fixed $T = 9.6$ $\mu$s, $f_1 \in \{1.2, 1.3\}$ MHz, and $q_1 \in$ {-0.125, -0.1042, -0.0833, -0.0625, -0.0417, -0.0208, -0.0104, -0.0052, 0} MHz$^2$. The signal was delivered to the NV via a loop of wire. The amplitude of the resulting magnetic field at the position of the interrogated NVs was on the order of 1.3 $\mu$T. For every pair $(f_1, q_1)$ a small delay on the order of 10-200 ns, presumably from the frequency-dependent impedence of the RF circuit, was calibrated to match the phase of the filter to that of the received signal. This step obviated the need to measure with in-quadrature ($\phi = \pi/2$) filters. The phases of successive $\pi$-pulses were cycled according to the XY8-N protocol [1, 2]. For every pair $(f_1, q_1)$ we performed a set of measurements for $f_j$ between 1 and 1.5 MHz with both matched chirp ($q = q_1$) and no chirp ($q = 0$), i.e. ordinary DD filters. The DD sequences described were nested between a $(\pi/2)_y$ pulse to initialize the NVs in the state $|+x\rangle = (|0\rangle + |1\rangle)/\sqrt{2}$, and a final $(\pi/2)_{\pm x}$ pulse to convert the acquired phase $\Phi$ into a population difference to be read out through the NV's spin-state-dependent fluorescence. This choice of initial and final pulse phases produces a measurement with contrast proportional to $\cos\Phi$. Ten iterations were recorded for each triple $(f_1, q_1, q)$. For every choice of filter we also recorded a background spectrum with the AWG

output turned off. A pulse generator (SpinCore Technologies, PBESR-PRO-500-PCI) was used to synchronize the AOM, microwave switch, detector, DAQ, IQ mixers, and arbitrary waveform generator. Hardware was controlled using custom MATLAB software. In practice it was easier to program each filter $h_j^{(\alpha)}$ to have a fixed number of pulses for all $j$ rather than fixed duration $T$. The effect on the resulting data is negligible and could be easily accounted for by using a $j$-dependent duration $T_j$ in our fitting model.

### B. Data Analysis

Each recorded spectrum was first background-corrected using a low-order polynomial fit of the recorded background spectrum for the corresponding filter. Contrast was computed as (signal-reference)/(signal+reference). For the estimation task depicted in Fig. 4(a) of the main text, we fit the vector of corrected contrasts $\mathscr{C}_j$ vs. $f_j$ for each trial to a model vector with elements of the form $\cos \Phi_j$, where $\Phi_j$ depends on the signal $g$ as described throughout this work. For both matched and unmatched filters we assumed $g$ of the form in Eq. (S1) with known $q_1$ and free parameters $A$ and $f_1$. Upon determining the best fit for $A$ and averaging over all trials, we fixed this number in the ensuing statistical analysis in order to focus attention on the estimation of $f_1$.

We empirically determined that the contrast was well-modeled as a Gaussian random variable with standard deviation $\sigma_{\mathscr{C}} = 0.1493$ by analysis of the pooled, corrected background data, which had an excess kurtosis of 0.1775 indicating approximate Gaussianity. Given the model $\mathscr{C}_j \sim \mathcal{N}\left(\cos\left[\Phi_j(f_1)\right], \sigma_{\mathscr{C}}^2\right)$, the Fisher information with respect to the scalar parameter $f_1$ is given by [3, 4]:

$$\mathcal{J}(f_1) = \sum_j \left[\frac{\Phi_j'(f_1)\sin\left[\Phi_j(f_1)\right]}{\sigma_{\mathscr{C}}^2}\right]^2. \tag{S2}$$

The associated Cramér-Rao bound given by

$$\sigma_{\mathrm{CRB}}^2(f_1) = \frac{1}{\mathcal{J}(f_1)} \tag{S3}$$

gives a lower bound to the variance of any unbiased estimator of $f_1$. For the set of $\{f_j\}$ chosen in our measurements we found that the least-squares estimates of $f_1$ derived from unmatched filters were significantly biased, and so comparison to the CRB is not necessarily appropriate. A Bayesian CRB which provides a lower bound to any estimator of $f_1$ is given by [4]:

$$\mathrm{MSE}_{\mathrm{BCRB}} \geq \frac{1}{\int \mathrm{d}f_1 p(f_1)\left[\mathcal{J}(f_1) + \left(\partial_{f_1}\log p(f_1)\right)^2\right]}, \tag{S4}$$

where $p(f_1)$ is a prior distribution on $f_1$. We heuristically found that $p(f_1)$ corresponding to a Gaussian of standard deviation $\sigma_{f_1} = 0.1$ MHz gives a reasonably tight bound. The BCRB values plotted in Fig. 4(a) are the means of the results computed for $f_1 = 1.2$ and $f_1 = 1.3$ MHz.

The binary hypothesis test depicted in Fig. 4(b) of the main text was carried out on each of the individual trials via a MAP test. Given our Gaussian noise model this amounts to choosing the hypothesis ($f_1 = 1.2$ MHz vs. $f_1 = 1.3$) which produces the smaller mean

squared error with respect to the observed data. The minimum probability of error for such a decision is sometimes called the Bayes error. When discriminating between two Gaussian processes possessing the same covariance matrix $\Sigma = \sigma^2 \mathbf{1}$ but different means $\vec{\mu}_0$ and $\vec{\mu}_1$, the Bayes error has a particularly simple analytical form given by [4]:

$$P_{\text{min error}} = \operatorname{erfc}\left(\frac{|\vec{\mu}_0 - \vec{\mu}_1|}{2\sigma}\right), \tag{S5}$$

with $\operatorname{erfc}(\cdot)$ denoting the complementary error function.

## II. RATIONALIZATION OF SUFFICIENT CONDITIONS FOR WHICH $\left|\Phi_j^{(\alpha)}\right|^2 \approx (4/\pi)^2 |\sin\alpha|\, |\mathcal{F}_\alpha[g](f_j \sin\alpha)|$

Consider the filter defined in the time domain by:

$$h_{j,\phi}^{(\alpha)}(t) = \operatorname{rect}\left(\frac{t - T/2}{T}\right) \tilde{h}_{j,\phi}^{(\alpha)}(t), \tag{S6}$$

with

$$\tilde{h}_{j,\phi}^{(\alpha)}(t) \equiv \operatorname{sgn}\left(\cos\left[2\pi t\left(-\frac{q}{2}t + f_j\right) - \phi\right]\right). \tag{S7}$$

The phase accumulated due to the signal $g$ under application of filter $h_{j,\phi}$ is:

$$\Phi_{j,\phi}^{(\alpha)} = \int g(t) h_{j,\phi}^{(\alpha)}(t)\mathrm{d}t. \tag{S8}$$

Suppose that we measure $\Phi_{j,0}^{(\alpha)}$ and $\Phi_{j,\pi/2}^{(\alpha)}$ directly and then take a complex linear combination to give:

$$\Phi_j^{(\alpha)} \equiv \Phi_{j,0}^{(\alpha)} - i\Phi_{j,\pi/2}^{(\alpha)}. \tag{S9}$$

We may view $\Phi_j^{(\alpha)}$ as the output of the signal with complex filter:

$$h_j^{(\alpha)}(t) \equiv h_{j,0}^{(\alpha)}(t) - i h_{j,\pi/2}^{(\alpha)}(t), \tag{S10}$$

that is:

$$\Phi_j^{(\alpha)} = \int g(t) h_j^{(\alpha)}(t)\mathrm{d}t. \tag{S11}$$

In this section we will sketch some sufficient (but not necessary) conditions for which $|\Phi_j^{(\alpha)}| \to (4/\pi)\sqrt{|\sin\alpha|}\, |\mathcal{F}_\alpha[g](f_j \sin\alpha)|$. First we will build some intuition. Using Parseval's relation we can rewrite:

$$\Phi_j^{(\alpha)} = \int \mathcal{F}_\alpha[g](u_\alpha)\, \mathcal{F}_\alpha^*\left[(h_j^{(\alpha)})^*\right](u_\alpha)\, \mathrm{d}u_\alpha, \tag{S12}$$

and so our ability to equate $\Phi_j^{(\alpha)}$ with the FRFT of $g$ depends on the extent to which $\mathcal{F}_\alpha^*\left[\left(h_j^{(\alpha)}\right)^*\right](u_\alpha)$ looks like a Dirac delta centered on $f_j \sin\alpha$. Figure S1 shows the absolute value of this quantity for a filter with $\alpha = \pi/2$, $f_j = 10$, and $T = 2.5$ (units arbitrary).

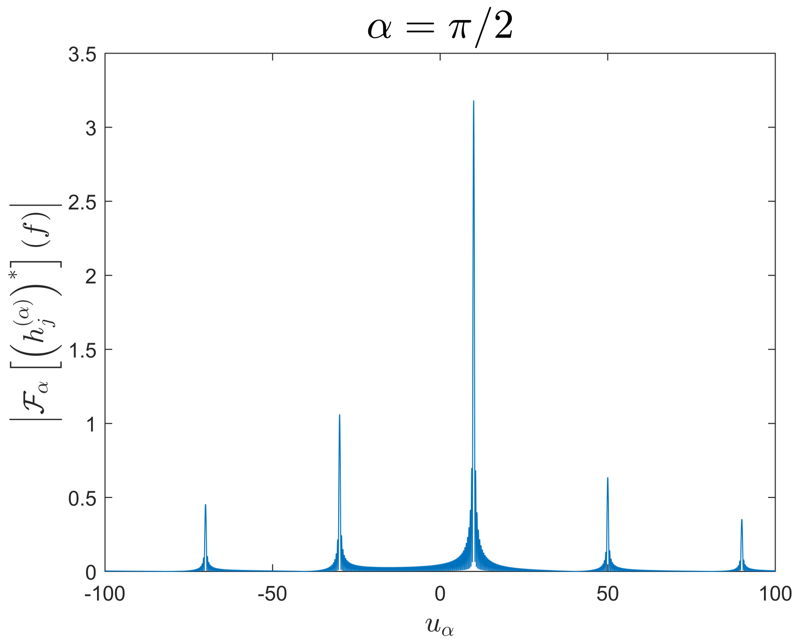


FIG. S1. Absolute value of FRFT of order $\alpha = \pi/2$ (i.e. the ordinary Fourier transfrom) of a filter with $f_j = 10$, $T = 2.5$, and $q = \cot\alpha = 0$ (units arbitrary).

Since $\alpha = \pi/2$ this corresponds to a conventional unchirped DD filter. The spectrum shows a global peak at $u_\alpha = f_j \sin\alpha = 10$, along with lower-amplitude peaks centered at $u_\alpha = (-1)^k(2k+1)f_j \sin\alpha$ for $k \in \mathbb{N}$. Contributions from the hamonics ($k \geq 1$) can be ignored if the energy of $g$ is concentrated near the fundamental. Figure S2 shows the same type of plot, except for $\alpha = \pi/4$. This spectrum shows a global peak at $u_\alpha = f_j \sin\alpha \approx 7$. There are features again near $u_\alpha = (-1)^k(2k+1)f_j \sin\alpha$ for $k \in \mathbb{N}$, but varying levels of chirp cause these features to spread out. We should be able to approximate this spectrum by the desired Dirac delta precisely when $\mathcal{F}_\alpha[g](u_\alpha)$ has minimal overlap with the chirped harmonics.

The absolute value of the acquired phase can also be written in terms of the Wigner functions of the signal and filter:

$$\left|\Phi_j^{(\alpha)}\right| = \left|\iint \mathrm{d}t\,\mathrm{d}f\, W_g(t,f) W_{h_j^{(\alpha)}}(t,f)\right|^{1/2} \tag{S13}$$

Possible shapes of these Wigner functions are sketched in Fig. S3 for $f_0 = 10$ (units arbitrary), $T = 2.5$ (units arbitrary), and either $\alpha = +\pi/10$ [Fig. S3(a)] or $\alpha = -\pi/10$ [Fig. S3(b)]. In these illustrations, black lines correspond to the centers of the fundamental and harmonics of $h_j^{(\alpha)}$, whereas the red bands correspond to possible signals which are sufficiently narrowly distributed around the fundamental such that the harmonics can be ignored. The red band is mirrored across $f = 0$ since we have specified throughout this work that $g(t)$ is real. Key features in this picture that make the desired approximation valid include the fact that the black line centered on the fundamental 1) does not cross $f = 0$ and 2) does not intersect with any of the harmonics on $t \in [0, T]$.

Having established this picture, let us now proceed with a more analysis-based approach.

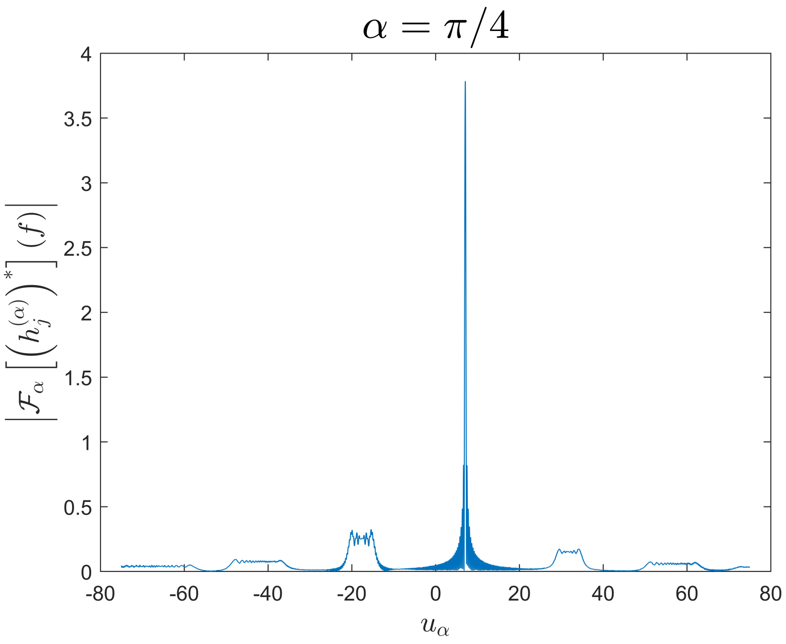


FIG. S2. Absolute value of FRFT of order $\alpha = \pi/4$ of a filter with $f_j = 10$, $T = 2.5$, and $q = \cot\alpha$ (units arbitrary).

Define:

$$\tilde{\Phi}_j^{(\alpha)} = \int g(t)\tilde{h}_j^{(\alpha)}(t)\mathrm{d}t, \tag{S14}$$

where

$$\tilde{h}_j^{(\alpha)}(t) \equiv \tilde{h}_{j,0}^{(\alpha)}(t) - i\tilde{h}_{j,\pi/2}^{(\alpha)}(t), \tag{S15}$$

in which case we can write:

$$\Phi_j^{(\alpha)} = \tilde{\Phi}_j^{(\alpha)} - \int_{-\infty}^{0} g(t)\tilde{h}_j^{(\alpha)}(t)\mathrm{d}t - \int_{T}^{\infty} g(t)\tilde{h}_j^{(\alpha)}(t)\mathrm{d}t. \tag{S16}$$

We will return to Eq. (S16) after introducing a bit more notation. Using the Fourier series relations:

$$\operatorname{sgn}(\cos u) = \sum_{k=0}^{\infty} \frac{4(-1)^k}{\pi(2k+1)} \cos\left[(2k+1)u\right] \tag{S17a}$$

$$\operatorname{sgn}(\sin u) = \sum_{k=0}^{\infty} \frac{4}{\pi(2k+1)} \sin\left[(2k+1)u\right] \tag{S17b}$$

we combine to write:

$$\begin{aligned}\tilde{h}_j^{(\alpha)}(t) &= \sum_{k=0}^{\infty} \frac{4(-1)^k}{\pi(2k+1)} e^{2\pi i(-1)^{k+1}(2k+1)\left[-\frac{q}{2}t^2+f_jt\right]} \\ &= \sum_{k=0}^{\infty} \tilde{h}_j^{(\alpha,k)}(t)\end{aligned} \tag{S18}$$

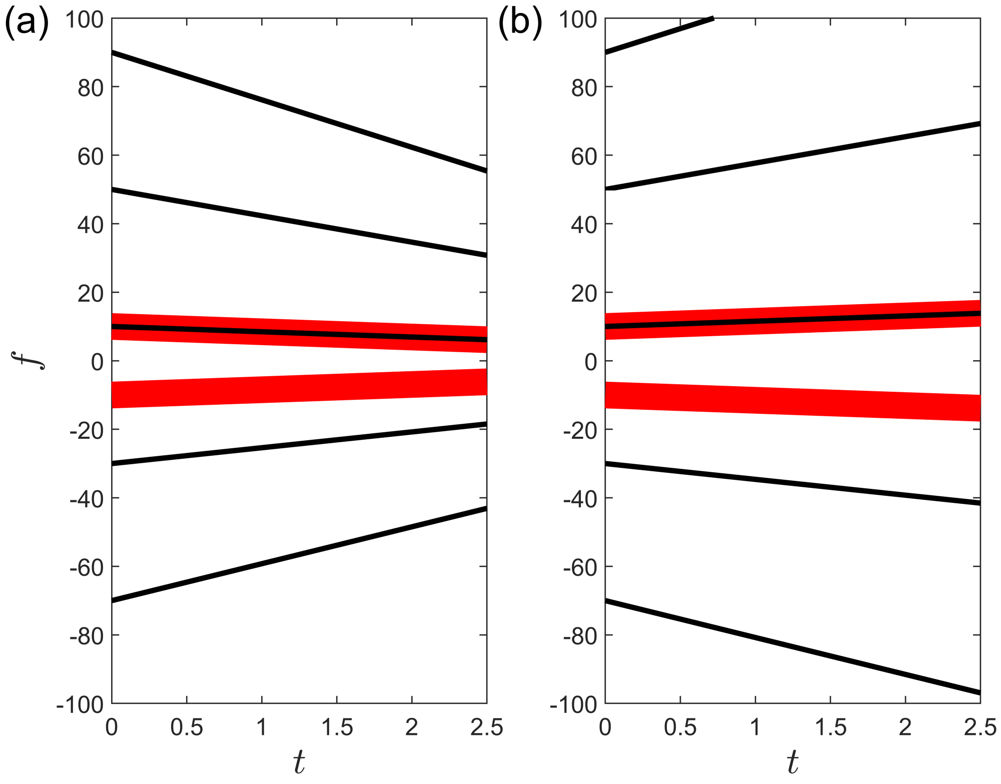


FIG. S3. Time-frequency sketches of filter and signal combinations for which the desired approximation is valid. Here $f_j = f_0 = 10$, $T = 2.5$, and $q = \cot\alpha$ (units arbitrary). Black lines correspond to the fundamental and harmonics of $h_j^{(\alpha)}$, while red bands correspond to the signal, $g$. (a) $\alpha = +\pi/10$ (down-chirped). (b) $\alpha = -\pi/10$ (up-chirped).

with

$$\tilde{h}_j^{(\alpha,k)}(t) \equiv \frac{4(-1)^k}{\pi(2k+1)} e^{2\pi i(-1)^{k+1}(2k+1)\left[-\frac{q}{2}t^2+f_j t\right]}. \tag{S19}$$

If we let

$$\tilde{\Phi}_j^{(\alpha,k)} \equiv \int g(t)\tilde{h}_j^{(\alpha,k)}(t)\mathrm{d}t, \tag{S20}$$

then

$$\tilde{\Phi}_j^{(\alpha)} = \sum_{k=0}^{\infty} \tilde{\Phi}_j^{(\alpha,k)} = \tilde{\Phi}_j^{(\alpha,0)} + \sum_{k=1}^{\infty} \tilde{\Phi}_j^{(\alpha,k)}. \tag{S21}$$

With these definitions now in hand we can rearrange Eq. (S16):

$$\Phi_j^{(\alpha)} - \tilde{\Phi}_j^{(\alpha,0)} = \sum_{k=1}^{\infty} \tilde{\Phi}_j^{(\alpha,k)} - \int_{-\infty}^{0} g(t)\tilde{h}_j^{(\alpha)}(t)\mathrm{d}t - \int_{T}^{\infty} g(t)\tilde{h}_j^{(\alpha)}(t)\mathrm{d}t. \tag{S22}$$

Applying the triangle inequality as well as the integral inequality $\left|\int \mathscr{G}(t)\mathrm{d}t\right| \leq \int |\mathscr{G}(t)|\,\mathrm{d}t$ to the RHS of Eq. (S22), and the reverse triangle inequality to the LHS of Eq. (S22), we

conclude:

$$\left| \left|\Phi_j^{(\alpha)}\right| - \left|\tilde{\Phi}_j^{(\alpha,0)}\right| \right| \leq \sum_{k=1}^{\infty} \left|\tilde{\Phi}_j^{(\alpha,k)}\right| + 2\int_{-\infty}^{0} |g(t)|\,\mathrm{d}t + 2\int_{T}^{\infty} |g(t)|\,\mathrm{d}t. \tag{S23}$$

If $g \in L^1$ we can choose the points $t = 0$ and $t = T$ such that the last two terms on the RHS of Eq. (S23) are arbitrarily small. Considering the $k = 0$ term:

$$\begin{aligned} \left|\tilde{\Phi}_j^{(\alpha,0)}\right| &= \frac{4}{\pi}\left|\int g(t)e^{-2\pi i\left[-\frac{q}{2}t^2+f_j t\right]}\right| \\ &= \frac{4\sqrt{|\sin\alpha|}}{\pi}\left|\mathcal{F}_\alpha[g](f_j \sin\alpha)\right|, \end{aligned} \tag{S24}$$

we can rewrite Eq. (S23):

$$\left| \left|\Phi_j^{(\alpha)}\right| - \frac{4\sqrt{|\sin\alpha|}}{\pi}\left|\mathcal{F}_\alpha[g](f_j \sin\alpha)\right| \right| \leq \sum_{k=1}^{\infty} \left|\tilde{\Phi}_j^{(\alpha,k)}\right| + 2\int_{-\infty}^{0} |g(t)|\,\mathrm{d}t + 2\int_{T}^{\infty} |g(t)|\,\mathrm{d}t. \tag{S25}$$

Thus if we can find some sufficient conditions under which the RHS of Eq. (S25) goes to 0 we will have achieved our goal. As we've established, we shouldn't expect for this to hold for general $g$, $\alpha$, and $f_j$. We do, however, expect it to hold in cases where the energy of $\mathcal{F}_\alpha[g](u_\alpha)$ is sufficiently localized to the vicinity around some $u_{\alpha,0} = f_0 \sin\alpha$ when $f_j$ is not too far from $f_0$. To make some progress in our analytical analysis we will now specify a particular form for $g$ that satisfies these requirements (as well as the requirement that $g(t)$ be real), with the obvious caveat that this will not be the only valid form for $g$ for which the desired approximation holds. Let:

$$g(t) = \cos\left[2\pi\left(-\frac{q}{2}t^2 + f_0 t\right) - \varphi\right] g_0(t), \tag{S26}$$

with

$$g_0(t) \equiv G_0 e^{-\frac{(t-T/2)^2}{2\tau^2}}, \tag{S27}$$

where $G_0, \varphi, \tau \in \mathbb{R}$ and $G_0, \tau > 0$. Centering the envelope at $t = T/2$ is equivalent to shifting our definition of the time origin to capture the important part of the wavepacket. Define:

$$\tilde{h}_j^{(\alpha,k,\pm)}(t) \equiv \tilde{h}_j^{(\alpha,k)}(t)e^{\pm 2\pi i\left[-\frac{q}{2}t^2+f_0 t-\frac{\varphi}{2\pi}\right]} \tag{S28}$$

and

$$\tilde{\Phi}_j^{(\alpha,k,\pm)} \equiv \int \tilde{h}_j^{(\alpha,k,\pm)}(t)g_0(t)\mathrm{d}t \tag{S29}$$

such that

$$\tilde{\Phi}_j^{(\alpha,k)} = \frac{\tilde{\Phi}_j^{(\alpha,k,+)} + \tilde{\Phi}_j^{(\alpha,k,-)}}{2}. \tag{S30}$$

Once again by application of the triangle inequality:

$$\left|\tilde{\Phi}_j^{(\alpha,k)}\right| \leq \frac{\left|\tilde{\Phi}_j^{(\alpha,k,+)}\right| + \left|\tilde{\Phi}_j^{(\alpha,k,-)}\right|}{2}. \tag{S31}$$

We can use the Moyal product property of the Wigner function [5, 6] to rewrite:

$$\left|\tilde{\Phi}_j^{(\alpha,k,\pm)}\right| = \left| \iint \mathrm{d}t\, \mathrm{d}f\, W_{\tilde{h}_j^{(\alpha,k,\pm)}}(t,f) W_{g_0}(t,f) \right|^{1/2}. \tag{S32}$$

The two Wigner functions in the integrand above have fairly simple forms. For one:

$$W_{\tilde{h}_j^{(\alpha,k,\pm)}}(t,f) = \frac{4}{\pi^2(2k+1)^2}\,\delta\left[f - \left(a^{(\alpha,k,\pm)}t + b_j^{(\alpha,k,\pm)}\right)\right], \tag{S33}$$

where

$$a^{(\alpha,k,\pm)} \equiv -q\left[(-1)^{k+1}(2k+1) \pm 1\right], \tag{S34a}$$

$$b_j^{(\alpha,k,\pm)} \equiv (-1)^{k+1}(2k+1)f_j \pm f_0. \tag{S34b}$$

The Wigner function of $g_0$ is given by:

$$W_{g_0}(t,f) = 2\sqrt{\pi}\tau G_0^2 \exp\left[-\frac{(t-T/2)^2}{\tau^2} - 4\pi^2\tau^2 f^2\right]. \tag{S35}$$

Plugging these into Eq. S32 and integrating gives:

$$\left|\tilde{\Phi}_j^{(\alpha,k,\pm)}\right| = \frac{\sqrt{8\tau}G_0}{\pi^{3/4}(2k+1)\left(\frac{1}{\pi\tau^2} + 4\pi\tau^2\left[a^{(\alpha,k,\pm)}\right]^2\right)^{1/4}} \exp\left[-\frac{\pi^2\tau^2\left(2b_j^{(\alpha,k,\pm)} + a^{(\alpha,k,\pm)}T\right)^2}{2\left(1+4\pi^2\tau^4\left[a^{(\alpha,k,\pm)}\right]^2\right)}\right]. \tag{S36}$$

More readily interpretable expressions can be obtained if we find a neater upper bound for the above equation. First note:

$$\frac{1}{\left(\frac{1}{\pi\tau^2} + 4\pi\tau^2\left[a^{(\alpha,k,\pm)}\right]^2\right)^{1/4}} \leq \frac{1}{\left(4\pi\tau^2\left[a^{(\alpha,k,\pm)}\right]^2\right)^{1/4}} = \frac{1}{\pi^{1/4}\sqrt{2\tau\left|a^{(\alpha,k,\pm)}\right|}}. \tag{S37}$$

Moreover, application of the reverse triangle inequality yields:

$$\left|a^{(\alpha,k,\pm)}\right| \geq 2|q|k. \tag{S38}$$

Substituting the two previous inequalities as well as $1/(2k+1) \leq 1/(2k)$ into Eq. (S36) gives:

$$\left|\tilde{\Phi}_j^{(\alpha,k,\pm)}\right| \leq \frac{G_0}{\pi\sqrt{2|q|}k^{3/2}}e^{-\xi}, \tag{S39}$$

where

$$\xi \equiv \frac{\pi^2\tau^2\left(2b_j^{(\alpha,k,\pm)}+a^{(\alpha,k,\pm)}T\right)^2}{2\left(1+4\pi^2\tau^4\left[a^{(\alpha,k,\pm)}\right]^2\right)}. \tag{S40}$$

The prefactor has been simplified. Next we will seek a simpler bound for the exponential part. Plugging in the definitions from Eq. (S34) gives:

$$\xi = \frac{2\pi^2\tau^2\Big(\left[(-1)^{k+1}(2k+1)f_j \pm f_0\right] - \frac{qT}{2}\left[(-1)^{k+1}(2k+1)\pm 1\right]\Big)^2}{1+4\pi^2\tau^4q^2\left[(-1)^{k+1}(2k+1)\pm 1\right]^2}. \tag{S41}$$

Let's say:

$$f_j = f_0 + \Delta f. \tag{S42}$$

Rearranging our expression for $\xi$ gives:

$$\xi = \frac{2\pi^2\tau^2\Big(\left[f_0-\frac{qT}{2}\right]\left[(-1)^{k+1}(2k+1)\pm 1\right] + \Delta f(-1)^{k+1}(2k+1)\Big)^2}{1+4\pi^2\tau^4q^2\left[(-1)^{k+1}(2k+1)\pm 1\right]^2}. \tag{S43}$$

Recognize that $f(T/2) = (f_0 - qT/2)$ is the instantaneous frequency of the carrier at the peak of the envelope. Let's assume $(f_0 - qT/2) > 0$ so that we can factor it out in the following way:

$$\begin{aligned}\xi &= \frac{2\pi^2\tau^2\left(f_0-\frac{qT}{2}\right)^2\Big(\left[(-1)^{k+1}(2k+1)\pm 1\right] + \frac{\Delta f}{f_0-\frac{qT}{2}}(-1)^{k+1}(2k+1)\Big)^2}{1+4\pi^2\tau^4q^2\left[(-1)^{k+1}(2k+1)\pm 1\right]^2} \\ &= \frac{2\pi^2\tau^2\left(f_0-\frac{qT}{2}\right)^2\left((-1)^{k+1}(2k+1)\left[1+\frac{\Delta f}{f_0-\frac{qT}{2}}\right]\pm 1\right)^2}{1+4\pi^2\tau^4q^2\left[(-1)^{k+1}(2k+1)\pm 1\right]^2}.\end{aligned} \tag{S44}$$

If we can find a lower bound for $\xi$ then we will have found an upper bound for $\exp(-\xi)$. We split the following argument into ones dealing with the numerator and denominator of $\xi$ as expressed in the second line of Eq. (S44), which we will denote $\mathrm{num}(\xi)$ and $\mathrm{den}(\xi)$, respectively. Application of the reverse triangle inequality to the factor on the far right of the numerator gives:

$$\mathrm{num}(\xi) \geq 2\pi^2\tau^2\left(f_0-\frac{qT}{2}\right)^2\left|(2k+1)\left|\left[1+\frac{\Delta f}{f_0-\frac{qT}{2}}\right]\right| - 1\right|^2. \tag{S45}$$

To enforce our intuition that $f_j$ shouldn't be too far from $f_0$, let's specify that $|\Delta f| < (f_0 - qT/2)/2$, in which case the term in square brackets above must be lie on the closed interval $[1/2, 3/2]$. The absolute value brackets can be dropped since the enclosed expression

is non-negative for $k \geq 1$. Also, under this assumption we have

$$\left((2k+1)\left[1+\frac{\Delta f}{f_0-\frac{qT}{2}}\right]-1\right) > 2k\left[1+\frac{\Delta f}{f_0-\frac{qT}{2}}\right], \tag{S46}$$

and therefore

$$\mathrm{num}(\xi) \geq 8\pi^2\tau^2k^2\left(f_0-\frac{qT}{2}\right)^2\left(1+\frac{\Delta f}{f_0-\frac{qT}{2}}\right)^2. \tag{S47}$$

We now return to $\mathrm{den}(\xi)$. The triangle inequality implies:

$$\mathrm{den}(\xi) \leq 1+4\pi^2\tau^4q^2\left(2k+2\right)^2 = 1+16\pi^2\tau^4q^2\left(k+1\right)^2. \tag{S48}$$

Combining Eqs. (S47) and (S48) yields:

$$\xi \geq \frac{8\pi^2\tau^2k^2\left(f_0-\frac{qT}{2}\right)^2\left(1+\frac{\Delta f}{f_0-\frac{qT}{2}}\right)^2}{1+16\pi^2\tau^4q^2\left(k+1\right)^2}. \tag{S49}$$

Dividing top and bottom by $k^2$ (which is fine since $k \geq 1$) gives:

$$\xi \geq \frac{8\pi^2\tau^2\left(f_0-\frac{qT}{2}\right)^2\left(1+\frac{\Delta f}{f_0-\frac{qT}{2}}\right)^2}{\frac{1}{k^2}+16\pi^2\tau^4q^2\left(1+\frac{1}{k^2}\right)^2}. \tag{S50}$$

The numerator of the RHS of Eq. (S50) is constant, while the denominator monotonically decreases with increasing $k$. Thus the supremum of the RHS is obtained in the limit $k \to \infty$ and we conclude:

$$\begin{aligned} \xi &\geq \frac{8\pi^2\tau^2\left(f_0-\frac{qT}{2}\right)^2\left(1+\frac{\Delta f}{f_0-\frac{qT}{2}}\right)^2}{16\pi^2\tau^4q^2} \\ &= \frac{\left(f_0-\frac{qT}{2}\right)^2\left(1+\frac{\Delta f}{f_0-\frac{qT}{2}}\right)^2}{2\tau^2q^2}. \end{aligned} \tag{S51}$$

Inserting this result into Eq. (S39) gives:

$$\left|\tilde{\Phi}_j^{(\alpha,k,\pm)}\right| \leq \frac{G_0}{\pi\sqrt{2|q|}k^{3/2}}\exp\left[-\frac{\left(f_0-\frac{qT}{2}\right)^2\left(1+\frac{\Delta f}{f_0-\frac{qT}{2}}\right)^2}{2\tau^2q^2}\right], \tag{S52}$$

and thus

$$\left|\tilde{\Phi}_j^{(\alpha,k)}\right| \leq \frac{G_0}{\pi\sqrt{2|q|}k^{3/2}}\exp\left[-\frac{\left(f_0-\frac{qT}{2}\right)^2\left(1+\frac{\Delta f}{f_0-\frac{qT}{2}}\right)^2}{2\tau^2q^2}\right], \tag{S53}$$

and

$$\sum_{k=1}^{\infty}\left|\tilde{\Phi}_j^{(\alpha,k)}\right| \leq \frac{G_0}{\pi\sqrt{2|q|}}\left(\sum_{k=1}^{\infty}k^{-3/2}\right)\exp\left[-\frac{\left(f_0-\frac{qT}{2}\right)^2\left(1+\frac{\Delta f}{f_0-\frac{qT}{2}}\right)^2}{2\tau^2q^2}\right] \tag{S54}$$

$$= \frac{G_0\,\zeta(3/2)}{\pi\sqrt{2|q|}}\exp\left[-\frac{\left(f_0-\frac{qT}{2}\right)^2\left(1+\frac{\Delta f}{f_0-\frac{qT}{2}}\right)^2}{2\tau^2q^2}\right], \tag{S55}$$

where $\zeta(\cdot)$ denotes the Riemann zeta function. We now have a useful expression to bound the first term on the RHS of Eq. (S25). With our assumed form of $g(t)$ we can also obtain neater bounds for the second and third terms of the RHS of Eq. (S25) in terms of the complementary error function, $\mathrm{erfc}(\cdot)$:

$$2\int_{-\infty}^{0}|g(t)|\mathrm{d}t \leq \sqrt{2\pi}G_0\tau\,\mathrm{erfc}\left(\frac{T}{2\sqrt{2}\tau}\right), \tag{S56}$$

and

$$2\int_{T}^{\infty}|g(t)|\mathrm{d}t \leq \sqrt{2\pi}G_0\tau\,\mathrm{erfc}\left(\frac{T}{2\sqrt{2}\tau}\right). \tag{S57}$$

Putting it all together gives:

$$\left|\left|\Phi_j^{(\alpha)}\right| - \frac{4\sqrt{|\sin\alpha|}}{\pi}\left|\mathcal{F}_\alpha[g](f_j\sin\alpha)\right|\right| \leq \frac{3G_0}{5\sqrt{|q|}}\exp\left[-\frac{\left(f_0-\frac{qT}{2}\right)^2\left(1+\frac{\Delta f}{f_0-\frac{qT}{2}}\right)^2}{2\tau^2q^2}\right] + 2\sqrt{2\pi}G_0\tau\,\mathrm{erfc}\left(\frac{T}{2\sqrt{2}\tau}\right), \tag{S58}$$

where we've also made use of the fact that $\zeta(3/2)/(\pi\sqrt{2}) \approx 0.59 < 3/5$. Finally, we normalize both sides of Eq. (S58) by the $L^1$-norm of $g_0(t)$, $\|g_0\|_1 = \sqrt{2\pi}G_0\tau$:

$$\frac{\left|\left|\Phi_j^{(\alpha)}\right| - \frac{4\sqrt{|\sin\alpha|}}{\pi}\left|\mathcal{F}_\alpha[g](f_j\sin\alpha)\right|\right|}{\|g_0\|_1} \leq \frac{3}{5\tau\sqrt{2\pi|q|}}\exp\left[-\frac{\left(f_0-\frac{qT}{2}\right)^2\left(1+\frac{\Delta f}{f_0-\frac{qT}{2}}\right)^2}{2\tau^2q^2}\right] + 2\,\mathrm{erfc}\left(\frac{T}{2\sqrt{2}\tau}\right). \tag{S59}$$

Keeping in mind the assumptions we invoked along the way, the RHS of Eq. (S59) can be made exponentially small for a given $\tau$ and $q$ if $T \gg \tau$ and $|f_0 - qT/2| \gg 0$, i.e. so long as the filter covers enough of the waveform and the mean carrier frequency of the signal is sufficiently high.

## III. DERIVATION OF THE SECOND MOMENT OF $\Phi$ IN RELATION TO $W_g$ FOR STOCHASTIC $g$

Let $g(t)$ be a real stochastic process and $h(t)$ be a real deterministic filter such that the accumulated phase

$$\Phi = \int g(t)h(t)\mathrm{d}t \tag{S60}$$

is itself a real random variable. The Wigner distributions of $g$ and $h$ are defined

$$W_g(t,f) \equiv \int \langle g\left(t+t'/2\right) g\left(t-t'/2\right)\rangle\, e^{-2\pi i f t'}\mathrm{d}t' \tag{S61}$$

and

$$W_h(t,f) \equiv \int h\left(t+t'/2\right) h\left(t-t'/2\right) e^{-2\pi i f t'}\mathrm{d}t'. \tag{S62}$$

Consider the overlap integral of these Wigner functions:

$$\begin{aligned}\iint \mathrm{d}t\,\mathrm{d}f\, W_g(t,f)W_h(t,f) = \iint \mathrm{d}t\,\mathrm{d}f \quad & \left[\left(\int \langle g\left(t+t'/2\right) g\left(t-t'/2\right)\rangle\, e^{-2\pi i f t'}\mathrm{d}t'\right)\right. \\ & \left.\times\left(\int h\left(t+t''/2\right) h\left(t-t''/2\right) e^{-2\pi i f t''}\mathrm{d}t''\right)\right].\end{aligned} \tag{S63}$$

So long as it's copacetic to exchange the order of integrals and distributional averaging we can rewrite:

$$\begin{aligned}\iint \mathrm{d}t\,\mathrm{d}f\, W_g(t,f)W_h(t,f) = \Bigg\langle \iiint \mathrm{d}t\,\mathrm{d}t'\,\mathrm{d}t''\, & g\left(t+t'/2\right) g\left(t-t'/2\right) \\ & \times h\left(t+t''/2\right) h\left(t-t''/2\right) \\ & \times\left(\int \mathrm{d}f\, e^{-2\pi i (t'+t'')f}\right)\Bigg\rangle.\end{aligned} \tag{S64}$$

Substituting the following relation

$$\delta\left(t'+t''\right) = \int \mathrm{d}f\, e^{-2\pi i (t'+t'')f} \tag{S65}$$

gives

$$\iint \mathrm{d}t\,\mathrm{d}f\, W_g(t,f)W_h(t,f) = \left\langle \iint \mathrm{d}t\,\mathrm{d}t'\, g\left(t+t'/2\right) g\left(t-t'/2\right) h\left(t+t'/2\right) h\left(t-t'/2\right)\right\rangle. \tag{S66}$$

A change of variables defined by $t_+ = t + t'/2$, $t_- = t - t'/2$ recasts the integral on the RHS:

$$\iint \mathrm{d}t\,\mathrm{d}f\, W_g(t,f) W_h(t,f) = \left\langle \iint \mathrm{d}t_+\,\mathrm{d}t_-\, g\left(t_+\right) g\left(t_-\right) h\left(t_+\right) h\left(t_-\right) \right\rangle \tag{S67}$$

$$= \left\langle \left( \int \mathrm{d}t_+ g(t_+) h(t_+) \right) \left( \int \mathrm{d}t_- g(t_-) h(t_-) \right) \right\rangle$$

$$= \left\langle \Phi^2 \right\rangle, \tag{S68}$$

and so indeed we conclude

$$\left\langle \Phi^2 \right\rangle = \iint \mathrm{d}t\,\mathrm{d}f\, W_g(t,f) W_h(t,f). \tag{S69}$$

## IV. TIME-FREQUENCY ILLUSTRATION OF THE EXPERIMENTAL MEASUREMENT

Figure S4 shows a time-frequency-plane illustration of the measurements presented in Fig. 3 of the main text. In the interest of highlighting the important features and suppressing spurious interference terms, the time-frequency distributions depicted here of the real-valued signal and filter correspond not to the Wigner distribution as defined in the main text, but rather to the variant sometimes called the "Wigner-Ville distribution" [7], $WV(t,f)$, which is defined for a real signal $s(t)$ by:

$$WV_s(t,f) \equiv \int s_a(t + t'/2) s_a^*(t - t'/2) e^{-2\pi i f t'} \mathrm{d}t', \tag{S70}$$

where $s_a(t)$ is the corresponding analytic signal given by:

$$s_a(t) \equiv s(t) + i\mathcal{H}[s(t)], \tag{S71}$$

with $\mathcal{H}$ denoting the Hilbert transform. The Wigner-Ville distribution does not possess the Moyal product property, but the fact that a large phase is expected when $WV_g$ and $W_{h_j}$ have significant overlap is nonetheless true in a qualitative sense.

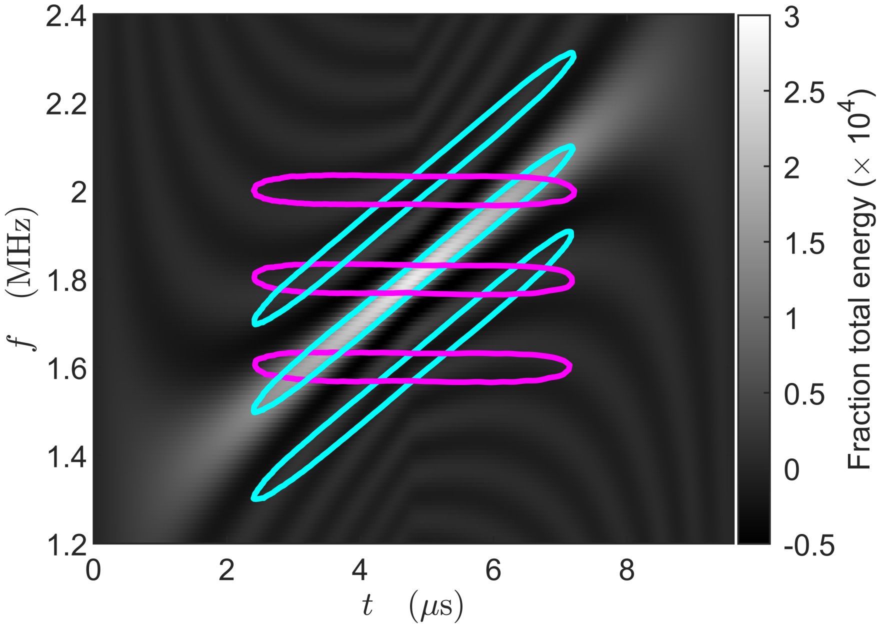


FIG. S4. Time-frequency illustration of the measurements presented in Fig. 3 of the main text. The grayscale image depicts $WV_g(t, f)$ for one particular choice of synthesized signal corresponding to $q_1 = -0.125$ MHz$^2$ and $f_1 = 1.25$ MHz. The contours corresponding to the half-maxima of $WV_{h_j}(t, f)$ with $f_j = (1.2 + 0.2j)$ MHz for $j \in \{-1, 0, 1\}$ are superimposed in cyan for $q = q_1$ and magenta for $q = 0$. In the $q = q_1$ case, $WV_{h_0}$ overlaps significantly while $WV_{h_{\pm 1}}$ overlap very little with $WV_g$, making for a sharp peak in the corresponding FRFT domain. For $q = 0$ each of the depicted $WV_{h_j}$ show partial overlap with the signal, translating to a low-amplitude, broad feature in the ordinary frequency domain.

[1] T. Gullion, D. B. Baker, and M. S. Conradi, Journal of Magnetic Resonance **89**, 479 (1990).
[2] A. M. Souza, G. A. Álvarez, and D. Suter, Phys. Rev. Lett. **106**, 240501 (2011).
[3] T. M. Cover and J. A. Thomas, *Elements of Information Theory* (John Wiley & Sons, 2005).
[4] H. L. Van Trees, *Detection, Estimation, and Modulation Theory, Part I: Detection, Estimation, and Linear Modulation Theory* (John Wiley & Sons, 2001).
[5] H. M. Ozaktas, Z. Zalevsky, and M. A. Kutay, *The Fractional Fourier Transform* (John Wiley & Sons, 2001).
[6] L. Cohen, *Time-Frequency Analysis* (Prentice Hall, 1995).
[7] A. Najmi, Johns Hopkins APL Technical Digest **15**, 298 (1994).
